# Supplementary material for: No-Regret Learning in Two-Echelon Supply Chain with Unknown Demand Distribution
Source: arXiv:2210.12663 source file (2023-10-20)
Supplement: Supplementary file 1 [file Appendix_experiment.tex]

\section{More empirical results}\label{app: experiments}
\input{Appendix_exp_decoupling}
\input{Appendix_exp_coupling}
